# Supplementary material for: Recovery Guarantees of Unsupervised Neural Networks for Inverse Problems trained with Gradient Descent
Source: arXiv:2403.05395 source file (2024-03-08)
Supplement: Supplementary file 1 [file appendix.tex]

\section{Reconstruction Bound in High Signal/Noise Ratio }\label{appendix:alternative_rec_bound}

The reconstruction bound given in \eqref{eq:xrate} relies on assumption~\ref{ass:F_inj} which requires injectivity of $\fopnl$ on $\Sigma$. An alternative way of deriving a similar bound only requires to impose restricted injectivity of the jacobian of $\fopnl$ at one point. The trade-off is that it is only valid for low noise level.

\begin{theorem}\label{thm:alternative_rec_bound}
    Under the setting of Theorem~\ref{thm:main}, let $\loss$ be convex and $\Argmin(\lossy(\cdot)) = \{\yv\}$. Assume that 
    \begin{assumption}\label{ass:F_jac_inj}
     %$\Jf$ is $\LJf$-Lipschitz continuous and
     $\ker(\Jf(\xvcsigma)) \cap T_{\Sigma'}(\xvcsigma) = {0}$.
    \end{assumption}
    Denote %$\xvinf = \lim_{t\rightarrow +\infty}\xvt$ and 
    \[
    \LF \eqdef \max_{\xv \in \Ball(0,2\norm{\xvc})} \norm{\Jf(\xv)} < +\infty . \quad \text{ and } \quad \delta(t) \eqdef \frac{2\psi\pa{\Psi\inv\pa{\gamma(t)}}}{\sigminjgz\sigminF} . %\LFtilde = \max_{\wv \in [\xvt,\xvcsigma]} \norm{\Jf(\wv)} < +\infty.
    \]
    Then for $\dist(\xvc,\Sigma')$ and $\norm{\varepsilon}$ small enough and all $t > 0$ sufficiently large, we have
    \begin{align}
    \norm{\xvt - \xvc} \leq \sqrt{\frac{\muf}{\LJf}\left(\frac{\LJf}{\muf} \dist(\xvc,\Sigma')^2 + \left(\frac{\LF}{\muf}+1\right)\dist(\xvc,\Sigma')+\frac{\delta(t) + \norm{\varepsilon}}{\muf}\right)} ,
    \end{align}
    where $\LJf > 0$ is a constant.

    %Let $\delta(t) \eqdef \frac{2\psi\pa{\Psi\inv\pa{\gamma(t)}}}{\sigminjgz\sigminF}$.
    %Furthermore, given $\delta > 0$, let $\tilde{t}$ be the time from which $\frac{2\psi\pa{\Psi\inv\pa{\gamma(t)}}}{\sigminjgz\sigminF} < \delta \quad \text{for all } t > \tilde{t}$.
    %Also assume that
    %\begin{align}\label{eq:real_pos_roots}
    %    \frac{\LJf}{\muf} \dist(\xvc,\Sigma)^2 + \left(\frac{\LJf}{\muf}+1\right)\dist(\xvc,\Sigma)+\frac{\delta + \norm{\varepsilon}}{\muf} \leq \frac{\muf}{4\LF}.
    %\end{align}
\end{theorem}

\begin{proof}
    Observe that Assumption~\ref{ass:F_jac_inj} implies that
    $\displaystyle{\muf = \lmin(\Jf(\xvcsigma);T_{\Sigma}(\xvcsigma))>0}$. Thus we have
    \begin{align*}
        \norm{\xvt - \xvc} &\leq \norm{\xvt - \xvcsigma} + \dist(\xvc,\Sigma')\\
        &\leq \muf\inv \norm{\Jf(\xvcsigma)(\xvt - \xvcsigma)} + \dist(\xvc,\Sigma').
    \end{align*}
    %We now argue similarly to the descent lemma~\cite[Lemma~2.64]{BauschkeBook} well-known in optimization. 
    Recall from Theorem~\ref{thm:main}\ref{thm:main_y_bounded} that $\theta(\cdot)$ is bounded, and therefore so is $\xv(\cdot)$ by continuity of $\gv(\uv,\cdot)$; i.e. $\xv(t) \in \Ball\pa{0,\rho}$ for some $\rho > 0$. It then follows from the local Lipschitz continuity assumption on $\Jf$ in \ref{ass:F_diff} that there exists $\LJf > 0$ such that for all $\zv, \zv^\prime \in \Ball\pa{0,\rho+2\norm{\xvc}}$
    \[
    \norm{\Jf(\zv)-\Jf(\zv^\prime)} \leq \LJf \norm{\zv-\zv^\prime} .
    \]
    In turn, we have
    \begin{align*}
    &\norm{\fopnl(\xvt)-\fopnl(\xvcsigma) - \Jf(\xvcsigma)(\xvt - \xvcsigma)}\\
    &= \norm{\int_0^1 \left(\Jf\left(\xvcsigma+t(\xvt - \xvcsigma)\right)-\Jf(\xvcsigma)\right)(\xvt - \xvcsigma) dt} \\
    &\leq \frac{\LJf}{2}\norm{\xvt - \xvc}^2 .
    \end{align*}
    Thus    
    \begin{align*}
         \norm{\xvt - \xvc} 
         %&\leq \muf\inv(\norm{\fopnl(\xvt) - \fopnl(\xvcsigma)} + \frac{1}{2}\max_{\wv \in [\xvt,\xvcsigma]}\norm{\Jf(\wv)}\norm{\xvt - \xvcsigma}^2) + \dist(\xvc,\Sigma)\\
         &\leq \muf\inv\left(\norm{\fopnl(\xvt) - \fopnl(\xvcsigma)} + \frac{\LJf}{2}\norm{\xvt - \xvcsigma}^2\right) + \dist(\xvc,\Sigma)\\
         &\leq \muf\inv(\norm{\yvt - \yv} + \norm{\fopnl({\xvcsigma}) - \yv} + \frac{\LJf}{2}\norm{\xvt - \xvcsigma}^2) + \dist(\xvc,\Sigma).
    \end{align*}
    From~\eqref{eq:klerrbnd}, we get
    \begin{multline*}
        \norm{\xvt - \xvc} 
        \leq \muf\inv(\delta(t) + \norm{\varepsilon} + \norm{\fopnl({\xvcsigma}) - \fopnl(\xvc)} + \LJf(\norm{\xvt - \xvc}^2 +  \dist(\xvc,\Sigma)^2)) \\
        + \dist(\xvc,\Sigma).
    \end{multline*}
    Using~\eqref{eq:diff_Fx_Fxsigma}, we obtain the following second-order polynomial inequality
    \begin{multline*}
        -\frac{\LJf}{\muf}\norm{\xvt - \xvc}^2 + \norm{\xvt - \xvc} \\ 
        - \muf\inv(\delta(t) + \norm{\varepsilon}) - \frac{\LJf}{\muf}\dist(\xvc,\Sigma)^2 - \left(1+\frac{\LF}{\muf}\right)\dist(\xvc,\Sigma) \leq 0.
    \end{multline*}
    Since $\delta(t) \to 0$, there exists $\tilde{t} > 0$ such that $\delta(t)$ is small enough for all $t \geq \tilde{t}$. Thus for all such $t$ and for sufficiently small $\dist(\xvc,\Sigma')$ and $\norm{\varepsilon}$, we know that the above polynomial has two real positive roots. Solving for $\norm{\xvt - \xvc}$, we get for $\dist(\xvc,\Sigma')$ and $\norm{\varepsilon}$ small enough and $t \geq \tilde{t}$, that
    \begin{align*}
        \norm{\xvt-\xvc} 
        &\leq \frac{\muf}{2\LJf} - \frac{\muf}{2\LJf}\left(\sqrt{1 - 4\frac{\LJf}{\muf}(\muf\inv(\delta(t)+\norm{\varepsilon}) + \frac{\LJf}{\muf}\dist(\xvc,\Sigma')^2 + \left(1+\frac{\LF}{\muf}\right)\dist(\xvc,\Sigma')}\right)\\
        &\leq \sqrt{\frac{\muf}{\LJf}(\muf\inv(\delta(t) + \norm{\varepsilon}) + \frac{\LJf}{\muf}\dist(\xvc,\Sigma')^2 + \left(1+\frac{\LF}{\muf}\right)\dist(\xvc,\Sigma')} .
    \end{align*}
\end{proof}

\section{Overparametrization Bound When the Linear Layer is Fixed}\label{appendix:V_fixed}

In the setting described in Section~\ref{sec:dip}, if one fixes the linear layer, as is usually done in the literature, a better overparametrization bound can be derived.

\begin{theorem}\label{th:dip_one_layer_fixed}%\label{th:dip_two_layers_converge}
Under the setting of Theorem~\ref{th:dip_two_layers_converge} where
\[
\LFz = \max_{\xv \in \Ball\pa{0,C\sqrt{n\log(d)}}} \norm{\Jf(\xv)}
\]
and
\[
\LLz = \max_{\vv \in \Ball\pa{0,C\LFz\sqrt{n\log(d)}+\sqrt{m}\pa{\norminf{\fopnl(\xvc)}+\norminf{\veps}}}} \frac{\norm{\nabla_\vv \lossy(\vv)}}{\norm{\vv-\yv}},
\]
consider the one-hidden layer network \eqref{eq:dipntk} where only the first layer is trained with the initialization satisfying \ref{ass:u_sphere}-\ref{ass:v_init} and the architecture parameters obeying
\begin{align*}
k \geq C' \sigminF^{-2} n \psi\pa{\frac{\LLz}{2}\pa{C\LFz \sqrt{n\log(d)} + \sqrt{m}\pa{\norminf{\fopnl(\xvc)} + \norminf{\veps}}}^2}^2 .
\end{align*}
Then \eqref{eq:bndR} holds with probability at least $1 - n^{-1} - d^{-1}$, where $C$ and $C'$ are positive constants that depend only on the activation function and $D$.
\end{theorem}

% discussion ?
%\begin{remark}\label{remark_fixed_linear}
%    The scaling of the overparametrization bound on $k$ with respect to $(n,m,d)$ in this setting with $\Vv$ fixed is such that $k\gtrsim \sigminF^{-2} n \psi(\LLz(\LFz^2 n + m))^2$. As a practical exemple, if we chose the loss to be the MSE and have an operator such that $\LFz$ is of constant order, we only need $k \gtrsim n^{2}m$. The main reason for such a change to happen in that setting is that by fixing $\Vv$, we remove the need to control the deviation of $\Vv$ from its initial point to obtain a local Lipschitz constant of the jacobian of the network. This allows to have a far better Lipschitz constant which is even global, consequently making $R$ less constrained.
%\end{remark}

\begin{proof}
The proof follows a very similar pattern as in the case where both layers are trained. The two main changes happen in the bounds on $\sigmin(\jthetaz)$ and $\Lip(\jcal)$. First, the constant on $\sigmin(\jthetaz)$ changes slightly but is still in $O(1)$ as described in lemma~\ref{lemma:min_eigenvalue_singvalue_init_one_layer}. The main change from the previous setting is that $\Lip(\jcal)$ is now a global constant given in lemma~\ref{lemma:lip-Jacobian-one-layer}. We now follow the same structure as in the proof of theorem~\ref{th:dip_two_layers_converge} and see that by Lemma~\ref{lemma:min_eigenvalue_singvalue_init_one_layer} and Lemma~\ref{lemma:lip-Jacobian-one-layer} we have that
\begin{align*}
    R \geq \frac{\Cphid}{2BD}\sqrt{\frac{k}{n}} \quad \text{thus,} \quad R \geq C_1\left(\frac{k}{n}\right)^{1/2}.
\end{align*}

Moreover, let us recall that by combining lemma~\ref{lemma:bound_initial_misfit} and the fact that
\[
[\yv,\yvz] \subset \Ball(0,\norm{\yv}+\norm{\yvz}) 
\]
we can deduce that with probability at least $1-n^{-1}$,
\[
\lossyzy \leq \frac{\LLz}{2}\pa{C\LFz \sqrt{n\log(d)} + \sqrt{m}\pa{\norminf{\fopnl(\xvc)} + \norminf{\veps}}}^2 .
\] 
Therefore, by using a union bound and that $\psi$ is increasing, for~\eqref{eq:bndR} to hold with probability $1 - n^{-1}-d^{-1}$, we need
\begin{align*}
    \sigminF^{-1} \psi\left(\frac{\LLz}{2}\pa{C\LFz \sqrt{n\log(d)} + \sqrt{m}\pa{\norminf{\fopnl(\xvc)} + \norminf{\veps}}}^2\right) \leq C_1\left(\frac{k}{n}\right)^{1/2}
\end{align*}
which gives the claim.
\end{proof}

\begin{lemma}[Bound on $\sigmin(\jthetaz)$]
\label{lemma:min_eigenvalue_singvalue_init_one_layer}
For the one-hidden layer network \eqref{eq:dipntk}, under assumptions \ref{ass:phi_diff} and \ref{ass:u_sphere} to \ref{ass:v_init}, we have
\begin{align*}
\sigmin(\jthetaz) \geq \Cphid/2 
\end{align*}
%with probability $1 - 2 \exp{(-c\tau^2)}$. Here, $C$, $c > 0$ depend only on the sub-gaussian norm $\normsubgauss{\phidW_1 \Vv_1}$ 
with probability at least $1-n^{-1}$ provided $k \geq C n\log(n)$ for $C > 0$ large enough that depends only on $\phi$ and the bound on the  entries of $\Vv$.
\end{lemma}

\begin{proof}
Define the matrix $\Hv = \jthetaz\jthetaz\tp$. For the two-layer network, and since $\uv$ is on the unit sphere, $\Hv$ reads
\[
\Hv = \frac{1}{k} \sum_{i=1}^k \phi'(\Wv^i(0)\uv)^2\Vv_i\Vv_i\tp .
\]
It follows that
\[
\Expect{}{\Hv} = \Expect{X\sim \stddistrib}{\phi'(X)^2}\frac{1}{k} \sum_{i=1}^k\Expect{}{\Vv_i \Vv_i\tp} = \Cphid^2 \Id_n ,
\]
where we used \ref{ass:u_sphere}-\ref{ass:w_init} and orthogonal invariance of the Gaussian distribution, hence $\Wv^i(0)\uv$ are iid $\stddistrib$, as well as \ref{ass:v_init} and independence between $\Vv$ and $\Wv(0)$. Moreover,
\[
\lammax(\phi'(\Wv^i(0)\uv)^2\Vv_i\Vv_i\tp) \leq B^2 D^2 n .
\]
We can then apply the matrix Chernoff inequality \cite[Theorem~5.1.1]{tropp_introduction_2015} to get
\[
\prob{\sigmin(\jthetaz) \leq \delta\Cphid} \leq ne^{-\frac{(1-\delta)^2k\Cphid^2}{2B^2 D^2 n}} .
\]
Taking $\delta=1/2$ and $k$ as prescribed, we conclude.
\end{proof}

\begin{lemma}[Global Lipschitz constant of $\jcal$ with linear layer fixed]\label{lemma:lip-Jacobian-one-layer}
Suppose that assumptions \eqref{ass:phi_diff}, \eqref{ass:u_sphere} and \eqref{ass:v_init} are satisfied. For the one-hidden layer network \eqref{eq:dipntk} with both layers trained, we have for $n \geq 2$ and any $\rho > 0$
\[
\Lip(\jcal) \leq BD \sqrt{\frac{n}{k}} .
\]
\end{lemma}

\begin{proof}
We have for all $\Wv, \Wvalt \in \R^{k \times d}$, 
\begin{align*}
\norm{\jW - \jWalt}^2 
&\leq \frac{1}{k} \sum_{i=1}^k |\phi'(\Wv^i\uv) - \phi'(\Wvalt^i\uv)|^2 \normf{\Vv_i\uv\tp}^2 \\
&=\frac{1}{k} \sum_{i=1}^k |\phi'(\Wv^i\uv) - \phi'(\Wvalt^i\uv)|^2 \norm{\Vv_i}^2 \\
&\leq B^2D^2\frac{n}{k} \sum_{i=1}^k |\Wv^i\uv - \Wvalt^i\uv|^2 \\
&\leq B^2D^2\frac{n}{k} \sum_{i=1}^k \norm{\Wv^i - \Wvalt^i}^2 = B^2D^2\frac{n}{k} \normf{\Wv - \Wvalt}^2 .
\end{align*}
\end{proof}
